# Supplementary material for: Bespoke Non-Stationary Solvers for Fast Sampling of Diffusion and Flow Models
Source: arXiv:2403.01329 source file (2024-03-02)
Supplement: Supplementary file 1 [file images_initial_solver_shutterstock_appendix.tex]

\begin{figure*}[t]
\centering
\begin{tabular}{@{\hspace{2pt}}c@{\hspace{1pt}}c@{\hspace{1pt}}c@{\hspace{1pt}}c@{\hspace{2pt}}@{\hspace{2pt}}c@{\hspace{1pt}}c@{\hspace{1pt}}c@{\hspace{1pt}}c@{\hspace{1pt}}c@{\hspace{0pt}}} 
{\scriptsize GT} & {\scriptsize NFE=20} & {\scriptsize NFE=16} & {\scriptsize NFE=12} & {\scriptsize GT} & {\scriptsize NFE=20} & {\scriptsize NFE=16} & {\scriptsize NFE=12} \\ 
% \rotatebox[origin=c]{90}{\scriptsize FM-OT}
\cincludegraphics[width=0.120 \textwidth]{example-grid-100x100pt} & 
    \begin{tabular}{@{\hspace{0pt}}c@{\hspace{0pt}}}    
        \includegraphics[width=0.120 \textwidth]{example-grid-100x100pt} \\
        \includegraphics[width=0.120 \textwidth]{example-grid-100x100pt}
    \end{tabular}
    &
    \begin{tabular}{@{\hspace{0pt}}c@{\hspace{0pt}}}   
        \includegraphics[width=0.120 \textwidth]{example-grid-100x100pt} \\
        \includegraphics[width=0.120 \textwidth]{example-grid-100x100pt}
    \end{tabular}
    &\begin{tabular}{@{\hspace{0pt}}c@{\hspace{0pt}}}  
        \includegraphics[width=0.120 \textwidth]{example-grid-100x100pt} \\
        \includegraphics[width=0.120 \textwidth]{example-grid-100x100pt}
    \end{tabular}
    &
\cincludegraphics[width=0.120 \textwidth]{example-grid-100x100pt} & 
    \begin{tabular}{@{\hspace{0pt}}c@{\hspace{0pt}}}   
        \includegraphics[width=0.120 \textwidth]{example-grid-100x100pt} \\
        \includegraphics[width=0.120 \textwidth]{example-grid-100x100pt}
    \end{tabular}
    &
    \begin{tabular}{@{\hspace{0pt}}c@{\hspace{0pt}}}
        \includegraphics[width=0.120 \textwidth]{example-grid-100x100pt} \\
        \includegraphics[width=0.120 \textwidth]{example-grid-100x100pt}
    \end{tabular}
    &\begin{tabular}{@{\hspace{0pt}}c@{\hspace{0pt}}}   
        \includegraphics[width=0.120 \textwidth]{example-grid-100x100pt} \\
        \includegraphics[width=0.120 \textwidth]{example-grid-100x100pt}
    \end{tabular}
    &\begin{tabular}{@{\hspace{0pt}}c@{\hspace{0pt}}}   
        \raisebox{2.2\height}{\rotatebox[origin=c]{90}{\scriptsize RK-Midpoint}} \\
        \raisebox{2.0\height}{\rotatebox[origin=c]{90}{\scriptsize BNS}}
    \end{tabular}
\end{tabular}
\caption{
    BNS vs. Intial solver
}\label{fig:a_t2i_bns_vs_initial_solver}
\end{figure*}
